# Supplementary material for: FlowerDance: MeanFlow for Efficient and Refined 3D Dance Generation
Source: arXiv:2511.21029 source file (2026-06-22)
Supplement: Supplementary file 1 [file X_suppl.tex]

\clearpage
\setcounter{page}{1}
\maketitlesupplementary

\appendix
\section{Implementation Details}
\noindent\textbf{Training Setup.}  
We adopt the Adan optimizer with a learning rate $4 \times 10^{-4}$, weight decay $0.02$, and default $\beta=(0.02,0.08,0.01)$. The model is trained for 4000 epochs with a batch size of 128 using the \text{Accelerate} library for distributed training on 4 NVIDIA RTX 3090 GPUs. We train on sequences of 240 frames (8s) and perform inference on sequences of 1024 frames (34.13s). EMA (decay $0.9999$) is applied to stabilize training, and checkpoints are periodically saved for evaluation. We combine multiple objectives:  MeanFlow loss ($\lambda_{mf}$=1), reconstruction loss ($\lambda_{rec}$=0.636), 3d joint position loss ($\lambda_{pos}$=0.636), and velocity loss ($\lambda_{vel}$=0.323).

\noindent\textbf{Model Architecture.}  
The conditional processing part contains 4 layers of BiMamba with Genre-Gate, and the vector generation part includes 8 layers of BiMamba-based block. Each Mamba unit uses $d_{\text{state}}=16$, convolutional kernel size $4$, and expansion factor $2$, and latent dimension $512$.

\section{Discussion about Sampling Strategy}
We investigate the effect of the sampling/ODE-solving strategy by comparing the simple Euler integrator~\cite{geng2025mean} with two classical higher-order schemes, Midpoint~\cite{hairer1993solving} and Heun~\cite{heun1900neue}. As reported in Tab.~\ref{tab: inference sample strategt}, our experiments show that, within the MeanFlow-based framework, the learned vector field corresponds to interval‑averaged velocities rather than instantaneous velocities. This mismatch violates the core assumption behind higher‑order solvers, which require accurate instantaneous velocity estimates at intermediate states. Consequently, re‑estimating velocities at these intermediate points with Midpoint or Heun introduces systematic errors that degrade sample quality. By contrast, the forward Euler—whose update is consistent with the interval‑averaged learning target—yields the best empirical performance across the evaluated metrics.

\begin{table}[h]
\centering

\setlength{\tabcolsep}{5pt}
\caption{Exploring the effect of Sampling Strategy.}
\vspace{-0.1in}
\label{tab: ablation}
\resizebox{\linewidth}{!}{
\begin{tabular}{l|ccc|cc|c}
\toprule
 & FID$_{k}$$\downarrow$ & FID$_{g}$$\downarrow$ & FSR$\downarrow$
 & Div$_{k}$$\uparrow$ & Div$_{g}$$\uparrow$
 & BAS$\uparrow$ \\

\midrule
Ground Truth   
& 0 & 0 & 21.62 
& 9.94 & 7.54 & 0.201
\\

Midpoint
& 49.78 & 65.47 & 0.402
& 8.75 & 7.05
& 0.217 \\

Huen
& 55.61 & 52.99 & 0.941
& 8.67 & 6.62
& \textbf{0.237} \\

Euler (Ours)
& \textbf{29.73} & \textbf{19.59} & \textbf{0.147}
& 8.42 & \textbf{7.18} & 0.232 \\

\bottomrule
\end{tabular}
}
\label{tab: inference sample strategt}
\vspace{-0.1in}
\end{table}

\section{Discussion about Foot Contact Loss}
Foot Contact Loss (FCL) has been widely adopted in prior works\cite{tseng2023edge,liu2025gcdance}, where the key idea is to predict binary foot contact labels and enforce the generated motion to remain consistent with these predictions, thereby reducing foot sliding artifacts. However, in our FlowerDance framework, we observe that incorporating FCL only improves Foot Sliding Ratio (FSR) while leading to negative effects on other evaluation metrics, as shown in Tab. \ref{tab: ccl}. More importantly, visual inspection reveals that FCL significantly reduces the diversity of generated dance movements and results in a "foot-locked" motion quality, where the footwork appears stiff and unnatural despite being grounded, as shown in Fig.~\ref{fig: ablation for fcl}.

Notably, while FCL has proven effective in diffusion-based motion generation models by progressively enhancing foot-contact stability over multiple sampling steps—thereby mitigating foot sliding without compromising overall motion quality—its direct transfer to our MeanFlow-based few-step generation framework yields suboptimal results. Although MeanFlow is not a single-step method, the number of generation steps is considerably fewer than in conventional diffusion models, forcing the model to simultaneously satisfy both global motion patterns and local contact constraints within a limited refinement window. In fact, our framework already incorporates SMPL- and joint-level constraints that implicitly enforce foot-contact stability, making this additional loss term less essential. Under such conditions, strong contact constraints are more likely to bias the global vector field distribution, thereby restricting diversity and naturalness and leading to performance degradation on other evaluation metrics.

%  你改一改这里就行了，把fig路径改一下
\begin{figure}[h]
  \centering
    \includegraphics[width=\linewidth]{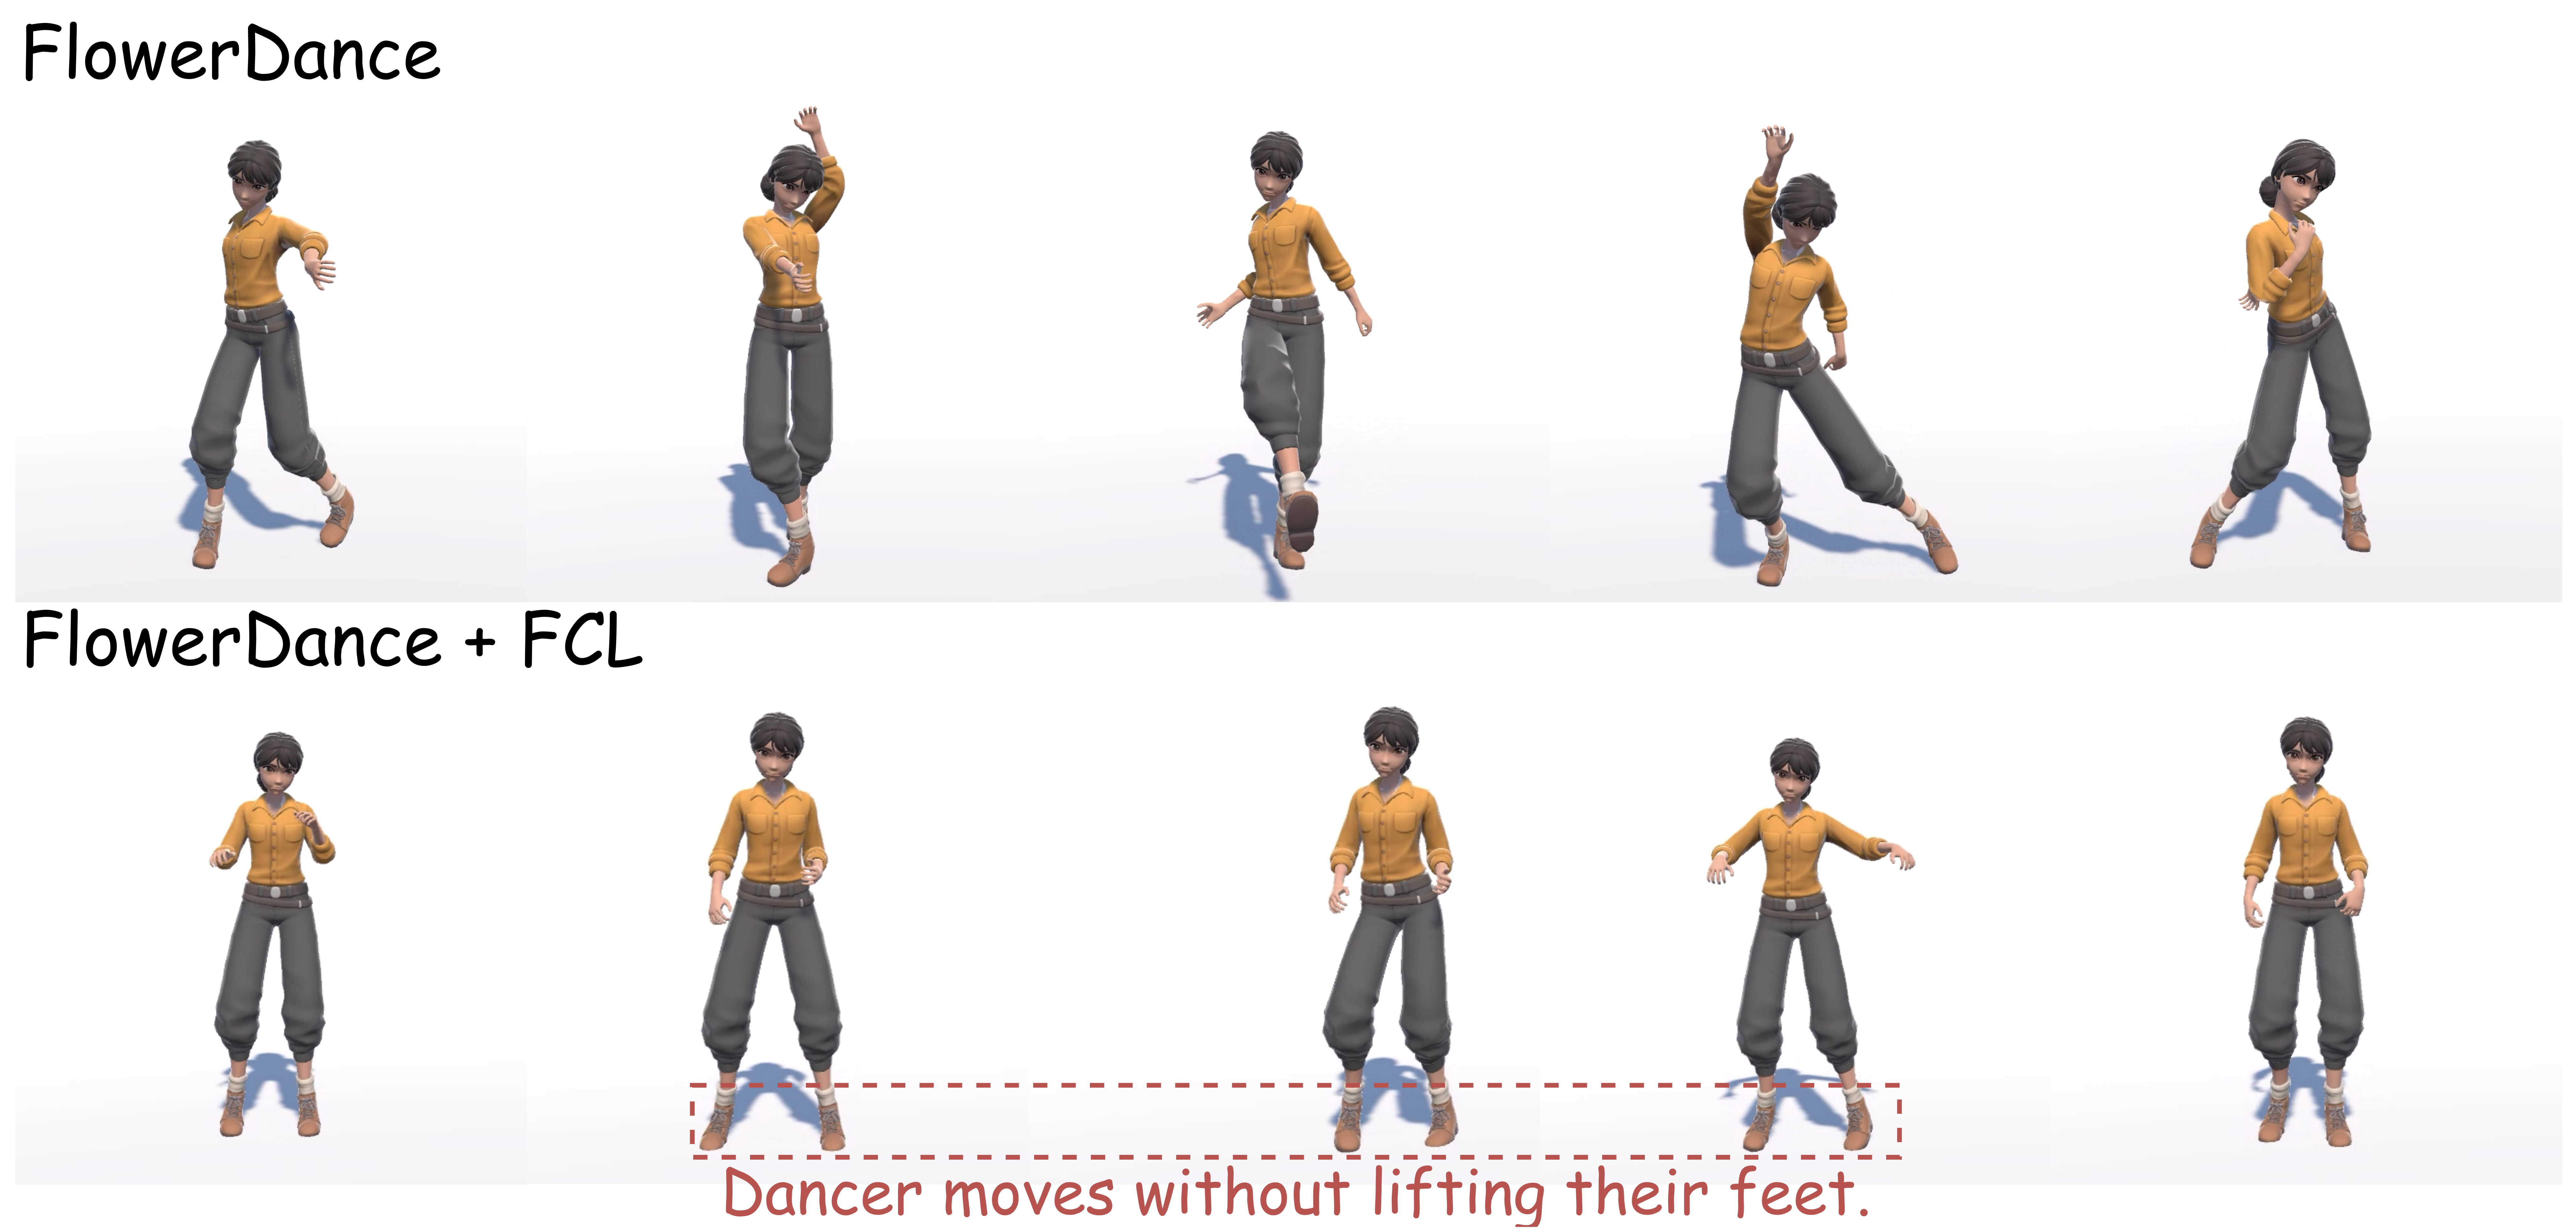}
  \caption{Ablation Study for foot contact loss (FCL).}
  \label{fig: ablation for fcl}
\end{figure}

\begin{table}[h]
\centering

\setlength{\tabcolsep}{5pt}
\caption{Exploring the effect of Foot Contact Loss (FCL).}
\vspace{-0.1in}
\label{tab: abl_fcl}
\resizebox{\linewidth}{!}{
\begin{tabular}{l|ccc|cc|c}
\toprule
 & FID$_{k}$$\downarrow$ & FID$_{g}$$\downarrow$ & FSR$\downarrow$
 & Div$_{k}$$\uparrow$ & Div$_{g}$$\uparrow$
 & BAS$\uparrow$ \\

\midrule
\small{Ground Truth}        
& 0 & 0 & 21.62 
& 9.94 & 7.54 & 0.201
\\
+ FCL
& 37.85 & 33.41 & \textbf{0.102}
& 7.36 & 6.91 & 0.211 \\
\textbf{FlowerDance}
& \textbf{29.73} & \textbf{19.59} & 0.147
& \textbf{8.42} & \textbf{7.18} & \textbf{0.232} \\

\bottomrule
\end{tabular}
}
\label{tab: ccl}
\vspace{-0.1in}
\end{table}

\section{Discussion about Classifier-Free Guidance}
Classifier-Free Guidance (CFG) is commonly employed to enhance conditional generation quality by combining conditional and unconditional predictions~\cite{tseng2023edge}. During training, the condition vector $\mathbf{c}$ is randomly dropped with probability $p \in [0.1, 0.2]$. During inference, the vector field is adjusted according to the guidance weight $\omega$, which determines the strength of conditional guidance:
\begin{equation}
u^{\text{cfg}}_\theta = \omega \cdot u_\theta(z_t, r, t \mid \mathbf{c}) 
+ (1-\omega)\cdot u_\theta(z_t, r, t \mid \varnothing),
\end{equation}

However, in the few-step generation setting, incorporating CFG tends to cause overshooting and introduce noticeable artifacts due to the absence of iterative refinement. As presented in Tab.~\ref{tab: cfg}, applying conventional CFG leads to a clear performance drop, with the increase in BAS largely attributable to high-frequency jittering errors. Visual inspection further indicates that CFG often induces random directional shaking and physically implausible poses. To address this issue, we investigate the recently proposed CFG-Zero$^{\star}$~\cite{fan2025cfg} and GFT~\cite{chen2025visual} (Guidance-Free Training), both of which have demonstrated strong results in image and video generation tasks. While these methods improve stability to some extent, they still exhibit occasional noticeable jitter and remain inferior to the original FlowerDance across all evaluation metrics. We acknowledge that CFG increases the diversity of generated dances and improves generalization to in-the-wild scenarios. However, the instability it introduces severely compromises motion quality, which is why we opted not to adopt it in FlowerDance. From another perspective, developing a suitable CFG strategy tailored to MeanFlow-based music-to-dance generation represents a valuable direction for future work.

\begin{table}[h]
\centering

\setlength{\tabcolsep}{5pt}
\caption{Exploring the effect of Classifier-Free Guidance (CFG).}
\vspace{-0.1in}
\label{tab: abl_cfg}
\resizebox{\linewidth}{!}{
\begin{tabular}{l|ccc|cc|c}
\toprule
 & FID$_{k}$$\downarrow$ & FID$_{g}$$\downarrow$ & FSR$\downarrow$
 & Div$_{k}$$\uparrow$ & Div$_{g}$$\uparrow$
 & BAS$\uparrow$ \\

\midrule
\small{Ground Truth}        
& 0 & 0 & 21.62 
& 9.94 & 7.54 & 0.201
\\
+ CFG
& 50.10 & 66.03 & 0.794
& \textbf{9.63} & 6.93 & \textbf{0.242} \\
+ CFG-Zero$^{\star}$
& \textbf{26.44} & 48.04 & 0.349
& 6.28 & 5.89 & 0.229 \\
+ GFT
& 32.96 & 35.86 & 0.187
& 8.37 & 7.06 & 0.238 \\
\textbf{FlowerDance}
& 29.73 & \textbf{19.59} & \textbf{0.147}
& 8.42 & \textbf{7.18} & 0.232 \\

\bottomrule
\end{tabular}
}
\label{tab: cfg}
\vspace{-0.1in}
\end{table}

\section{Questionnaire Details for User Study}
User feedback is essential for evaluating generated dance movements in the music-to-dance generation task, due to the inherent subjectivity of dance ~\cite{legrand2009perceiving}. Following \cite{yang2025megadance}, we select 30 real-world music segments, each lasting 34 seconds, and generated dance sequences using the models described above. These sequences are evaluated through a double-blind questionnaire completed by 40 participants with dance backgrounds, including undergraduate and graduate students. Participants are compensated at a rate exceeding the local average hourly wage. The questionnaires used a 5-point scale (Great, Good, Fair, Bad, Terrible) to assess three aspects: Dance Synchronization (DS, alignment with rhythm and style), Dance Quality (DQ, biomechanical plausibility and aesthetics), and Dance Creativity (DC, originality and range). The screenshot of our user study website is shown in Fig. \ref{fig: user study questionnaire}, displaying the template layout presented to the participants. In addition to the main trials, participants are also subjected to several catch trials, which involved displaying Ground Truth videos and videos with distorted motion. Participants who failed to rate the GT videos higher and the distorted motion videos lower are considered unresponsive or inattentive, and their data are excluded from the final evaluation.

\begin{figure}[h]
  \centering
\includegraphics[width=0.75\linewidth]{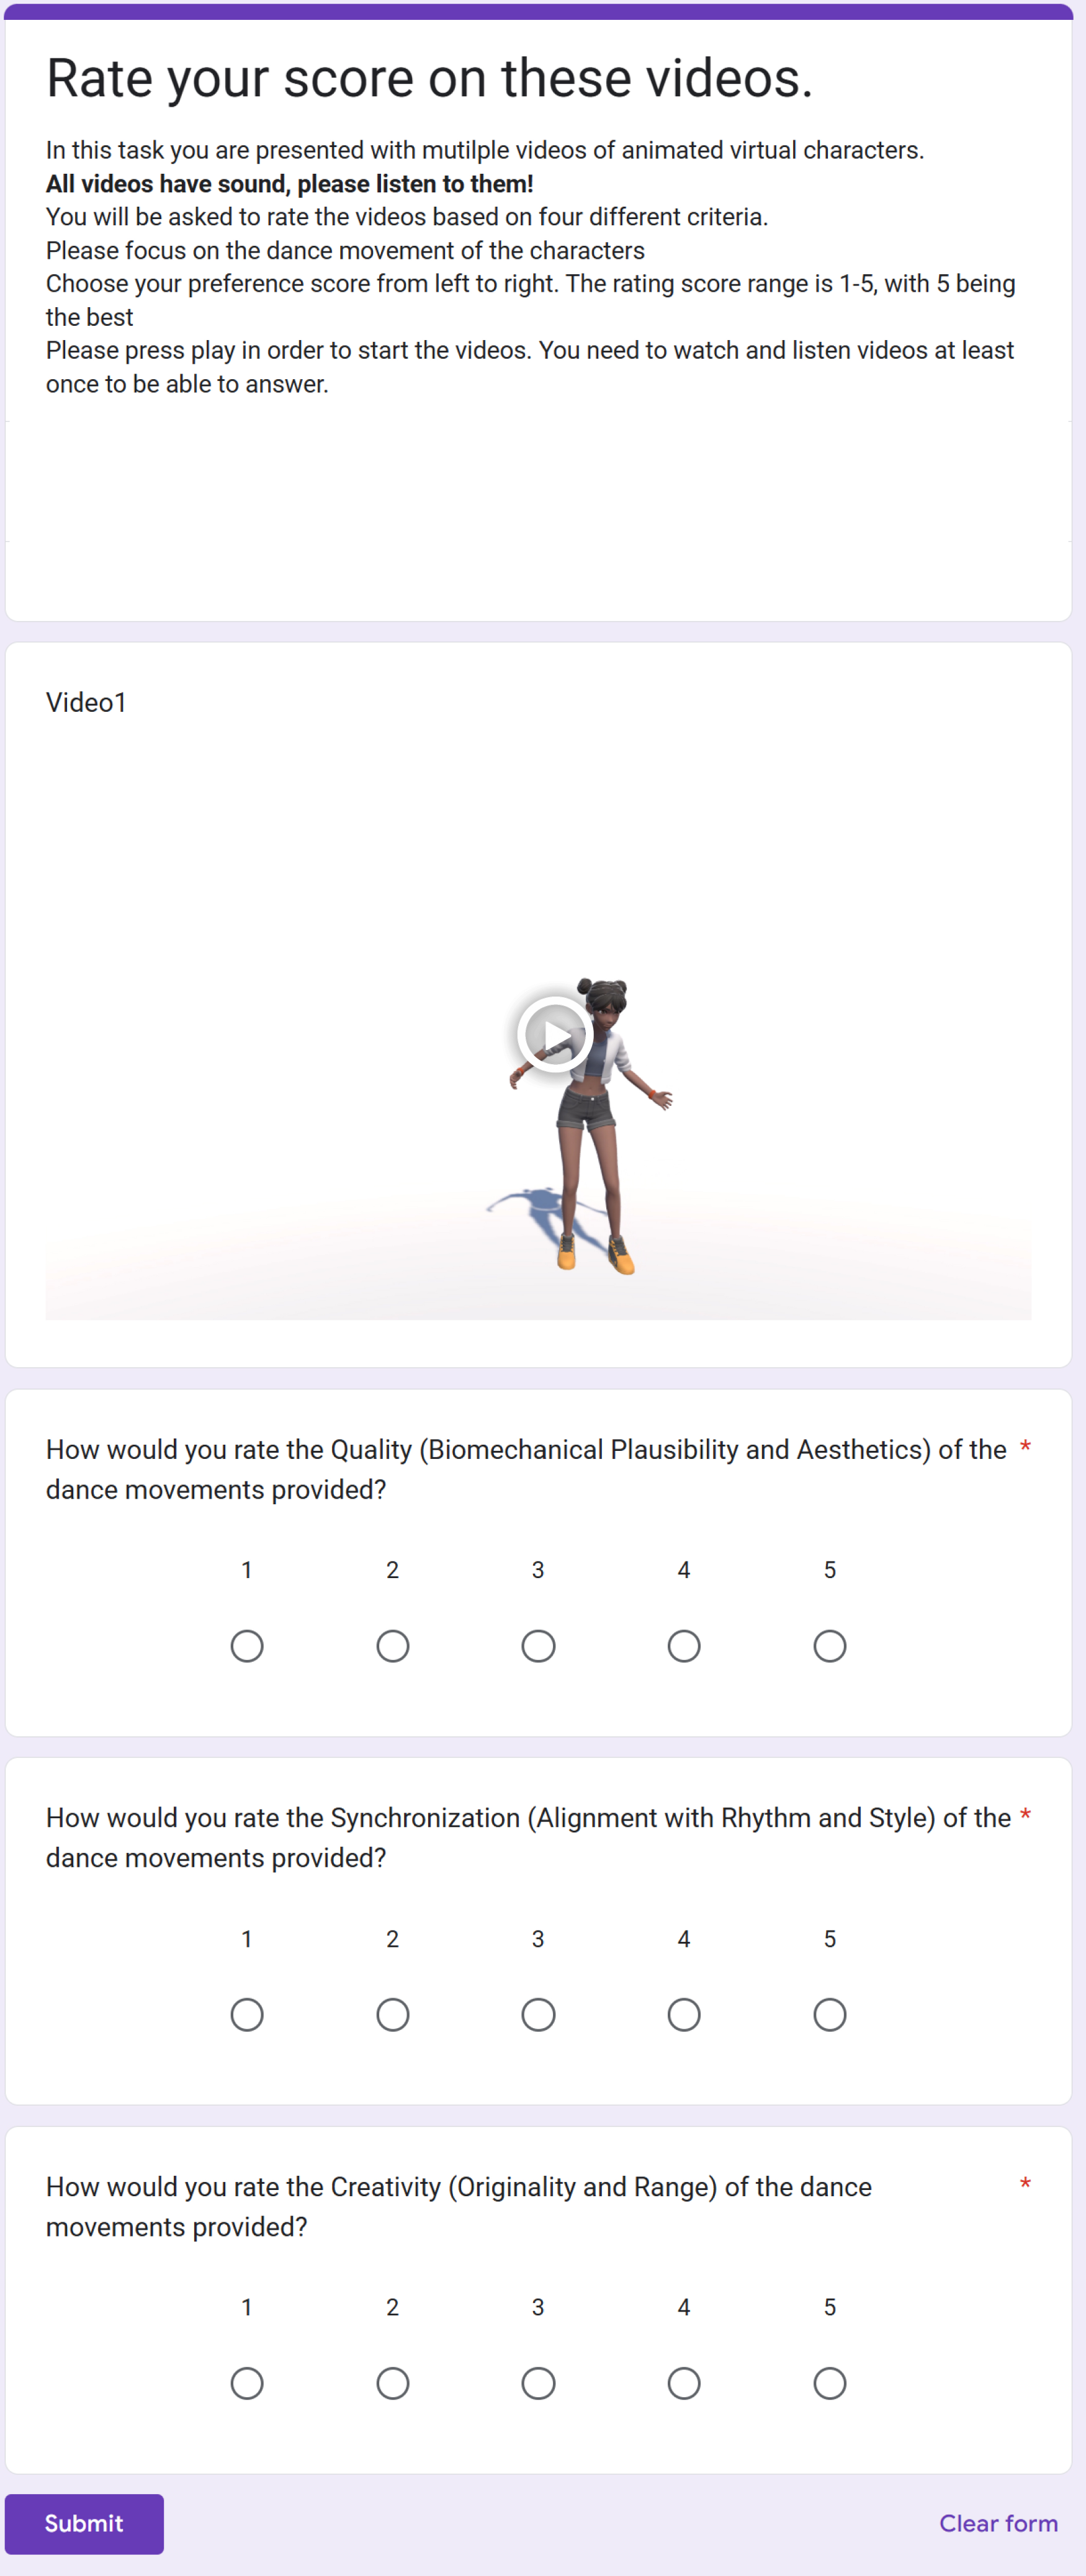}
  \caption{The screenshots of user study website for participants.}
  \label{fig: user study questionnaire}
\end{figure}

\begin{figure*}[t]
    \centering

    % 第一张
    \includegraphics[width=\linewidth]{}
    \caption{Temporal motion editing visualization. Green indicates the given motion, while yellow indicates the FlowerDance‑generated motion. (a) Middle segment given, sides completed; (b) Sides given, middle completed.}
    \label{fig:me1}

    \vspace{1em}

    % 第二张
    \includegraphics[width=\linewidth]{}
    \caption{Joint-level motion editing visualization. White indicates the provided motion, and black indicates the FlowerDance-generated motion. (a) Upper body given, lower body completed; (b) Lower body given, upper body completed.}
    \label{fig:me2}

    \vspace{1em}

    % 第三张
    \includegraphics[width=\linewidth]{}
    \caption{Trajectory‑based motion editing visualization. (a) FlowerDance‑generated dance with a given S‑shaped trajectory; (b) FlowerDance‑generated dance with a given C‑shaped trajectory.}
    \label{fig:me3}

\end{figure*}

\section{Details about Motion Edition}
It is widely acknowledged that motion editing is an essential step in dance generation, allowing users to refine results through interactive control. Extending the idea of inpainting in diffusion-based motion generation~\cite{liu2025gcdance,tseng2023edge}, FlowerDance also provides flexible motion editing capabilities during the sampling stage without additional training cost. 
Specifically, our motion editing supports three levels of control: \textbf{temporal}, \textbf{joint-level}, and \textbf{trajectory-level}, as illustrated in Figures~\ref{fig:me1}--\ref{fig:me3}.  
In the \emph{temporal} level (Fig.~\ref{fig:me1}), users can provide motion segments either at the middle or the sides of a sequence, with the remaining frames completed by the model.  
In the \emph{joint-level} editing (Fig.~\ref{fig:me2}), users can fix specific body parts, such as the upper or lower body, while FlowerDance generates the motion for the remaining joints to ensure consistent whole-body dynamics.  
At the \emph{trajectory-level} (Fig.~\ref{fig:me3}), users can define global motion paths, such as S-shaped or C-shaped trajectories, and FlowerDance synthesizes dance sequences that faithfully follow the given spatial constraints while preserving motion quality.

% \begin{figure*}[h]
%     \centering
%     \includegraphics[width=0.9\linewidth]{figs/me_1.pdf}
%     \caption{Temporal motion editing visualization. Green indicates the given motion, while yellow indicates the FlowerDance‑generated motion. (a) Middle segment given, sides completed; (b) Sides given, middle completed.}
%     \label{fig: me_1}
%     \vspace{-0.2in}
% \end{figure*}

% \begin{figure*}[h]
%     \centering
%     \includegraphics[width=0.9\linewidth]{figs/me_2.pdf}
%     \caption{Joint-level motion editing visualization. White indicates the provided motion, and black indicates the FlowerDance-generated motion. (a) Upper body given, lower body completed; (b) Lower body given, upper body completed.}
%     \label{fig: me_2}
%     \vspace{-0.2in}
% \end{figure*}

% \begin{figure*}[t]
%     \centering
%     \includegraphics[width=0.9\linewidth]{figs/me_3.pdf}
%     \caption{Trajectory‑based motion editing visualization. (a) FlowerDance‑generated dance with a given S‑shaped trajectory; (b) FlowerDance‑generated dance with a given C‑shaped trajectory.}
%     \label{fig: me_3}
%     \vspace{-0.2in}
% \end{figure*}

\section{Limitations and Future Work.}
\noindent\textbf{Customized Dance Generation.}
Although our FlowerDance framework achieves strong performance in music-to-dance generation and provides a motion-editing interface for user interaction, both music and motion-editing modalities have inherent limitations. Music serves as a fixed-form carrier and cannot fully capture diverse user intentions, while motion editing requires access to 3D motion capture devices or high-precision pose estimation algorithms, incurring considerable costs. To address these limitations, we envision extending control modalities to incorporate free-form textual descriptions. Text offers the lowest-cost input modality while allowing users to express choreographic requirements in a more flexible and semantically rich manner, thereby facilitating personalized and expressive dance generation. This direction not only enhances user interactivity and creativity but also unlocks new opportunities for content-driven applications in virtual performance and human–computer interaction. While recent studies have explored text-controlled dance generation, current approaches are hindered by the limited scale of available 3D training data and the difficulty in acquiring textual descriptions that not only align with natural user expression patterns but also semantically and precisely reflect the essential characteristics of dance movements.

\noindent\textbf{Noise-Resistant Dance Generation.}
3D motion capture data are often affected by noise artifacts, such as sudden positional jumps or temporal discontinuities, even in high-quality datasets like FineDance~\cite{li2023finedance} and AIST++~\cite{li2021ai}. Although some studies have proposed alignment-based refinement methods, these approaches remain insufficient to fully address the issue~\cite{mu2025stablemotion}. Moreover, the limited scale of existing 3D dance datasets makes models more susceptible to overfitting, further amplifying the problem. Future research should explore more robust architectures and data augmentation strategies that can preserve motion plausibility and stylistic coherence under noisy or incomplete inputs, thereby improving the reliability and generalization of music-to-dance generation systems.
